# Supplementary material for: Gradient Inversion of Federated Diffusion Models
Source: arXiv:2405.20380 source file (2024-05-30)
Supplement: Supplementary file 1 [file appendix.tex]

\section{Setups and details}
\subsection{Experimental setups}
\label{app:setup}

\textbf{Hardware.} For hardware, we conducted our experiments using an Alienware Aurora R13 running Ubuntu 20.04. This system boasts 64GB of memory, a GeForce RTX 3090 GPU, and a 16-core Intel i9 CPU. With each of its 8 P-cores supporting two threads, the machine houses a total of 24 logical CPU cores.

\textbf{Implement.} The project of this paper is based on Pytorch 2.3.0. In our gradient inversion attackers, we apply Adam as the optimizer for both $\boldsymbol{\epsilon}$, $t$ and the dummy image. The learning rate used in this paper is $0.01$ without any scheduler for learning rate decay. The diffusion model for our experiments is the commonly used DDPM which uses UNet to implement the sampling of each step. In our topic, the number of clients in the Federated learning system won't affect the results. 

\textbf{Dataset. }The \textit{CelebA} dataset~\cite{celebA:conf/iccv/LiuLWT15} is a widely used dataset in the computer vision community for tasks like face recognition, facial attribute analysis, and facial key points detection. It contains over 200,000 celebrity images with annotations for 40 facial attributes such as gender, age, hair color, and more. Each image is a high-quality RGB image and the dataset is well-suited for training and benchmarking computer vision algorithms related to facial analysis tasks.  The CelebA dataset images have an original size of $178 \time 218$ pixels. However, these images are often cropped and resized to 128x128 pixels or 64x64 pixels, depending on the requirements of the specific machine-learning tasks or models being used. The cropping is usually centered on the face to ensure that the primary subject of each image remains prominent.

The \textit{LSUN-Bedroom} dataset is a large collection of approximately 3 million bedroom images used for training and evaluating machine learning models in computer vision. The original dataset contains high-resolution images, but $256 \times 256$ is a common size used in practice to balance detail and computational efficiency. It features a wide variety of bedroom styles and conditions, making it ideal for tasks like image classification, scene recognition, and generative modeling. The dataset is especially popular for training Generative Adversarial Networks (GANs) and serves as a standard benchmark for evaluating the performance of various algorithms in scene understanding and image generation.

The \textit{CIFAR-100} dataset is a widely used benchmark dataset in machine learning and computer vision. It consists of 60,000 32x32 color images across 100 different classes, with each class containing 600 images. The dataset is divided into 50,000 training images and 10,000 test images. Each class in CIFAR-100 is further grouped into 20 superclasses, making it a more fine-grained and challenging dataset compared to CIFAR-10. The CIFAR-100 dataset is used for tasks such as image classification and object recognition, helping to evaluate and compare the performance of various algorithms.

\textbf{Baseline translation.} For the same training input of images, DLG-dm and InvG-dm choose the same dimensional dummy image as DLG and InvG for the optimization target. As the backpropagation on calculating the gradients processes the inference phase, which requires additional inputs of $\boldsymbol{\epsilon}$ and $t$, for DLG-dm and InvG, we randomly sample $\boldsymbol{\epsilon}$ following Gaussian distribution of the same size of the dummy image, and $t$ from $[1, T]$ following a uniform distribution. They are set constant during multiple inversion iterations. When it comes to the distance metric, we keep L2-Norm for DLG-dm and cosine similarity for InvG-dm respectively, which are consistent with DLG and InvG.

\subsection{Threat model}
\label{app:threat}
Our threat model considers the federated server $\mathcal{S}$ as the adversarial to reconstruct the input training data $X_k$ of the target client $C_k$. The threat model is described as follows.

\textbf{Objective.} The adversarial server aims to recover the input data $X_k$ trained on Client $C_k$ based on the gradient $g_k = \nabla_\theta\left\|\boldsymbol{\epsilon}_k-\boldsymbol{\epsilon}_{\theta_k}\left(\sqrt{\bar{\alpha}_t} \mathbf{x}_0+\sqrt{1-\bar{\alpha}_t} \boldsymbol{\epsilon}_k, t\right)\right\|^2$ during a specific global training round $r$. As the inversion can be executed at one given global round, we ignore the $r$ index for simplicity. The attack is successful if the recovered image $\hat{X}$ is almost identical to $X_k$.

\textbf{Capability.} We assume that the honest-but-curious servers do not have access to the real data of data owners. On the other hand, the
servers’ computational resources are bounded.

\textbf{Knowledge.} To recover input data at the specific round, we assume $\mathcal{S}$ naturally owns the global model and can access the model parameters and the submitted gradient by each client. However, the initialization of $\epsilon$ and the sampling step of $t$ are unknown to the adversary.

\subsection{Privacy defenses of federated learning systems.} 
In order to enhance system privacy against privacy leakage attacks and not significantly reduce model accuracy~\cite{gradprune:conf/eccv/YeDLGQYC20,sparsity:conf/emnlp/AjiH17,dropout:journals/corr/abs-1207-0580,Soteria:conf/cvpr/Sun0WY0C21}, current defenses are primarily conducted individually, falling into two categories: gradient perturbation and input perturbation. Gradient perturbation~\cite{gradprune:conf/eccv/YeDLGQYC20,gradprune:conf/icml/SunRMW17,dp:conf/tcc/Dwork09,dpsgd:conf/ccs/AbadiCGMMT016,sparsity:conf/emnlp/AjiH17,dropout:journals/corr/abs-1207-0580,dropout:journals/jmlr/SrivastavaHKSS14,graddrop:conf/nips/HuangGSLA21}, preferred for its efficiency and maintaining global model accuracy, involves transmitting perturbed gradients. In contrast, input perturbation, such as mixing images before local training, is less common~\cite{mixup:conf/iclr/ZhangCDL18}.
Prominent gradient perturbation defenses include differential private stochastic gradient descent~\cite{dp:conf/tcc/Dwork09}, which adds noise and clips gradients to limit sensitivity~\cite{dpsgd:conf/ccs/AbadiCGMMT016}. Gradient sparsification accelerates training by setting small gradient entries to zero~\cite{sparsity:conf/emnlp/AjiH17}, differing from dropout by removing small entries rather than randomly selecting them~\cite{graddrop:conf/nips/HuangGSLA21,dropout:journals/corr/abs-1207-0580,dropout:journals/jmlr/SrivastavaHKSS14}. Soteria proposes a fully-connected defense layer to perturb data representation, crucial for preventing inversion attacks while preserving Federated Learning performance~\cite{Soteria:conf/cvpr/Sun0WY0C21}.
Overall, defense efficacy factors on parameters like noise level, clipping bound, sparsity, and pruning rate, which need to be carefully chosen to balance model quality and privacy.

\subsection{Evaluation metrics}
\label{app:metric}
In evaluating the gradient inversion attack, which aims to reconstruct data that closely matches the original client data, we employ four metrics to gauge the resemblance between the reconstructed and real data: Mean Squared Error (MSE), Structural Similarity Index (SSIM)\cite{ssim:journals/tip/WangBSS04}, Peak Signal-to-Noise Ratio (PSNR)\cite{psnr:conf/icpr/HoreZ10}, and Learned Perceptual Image Patch Similarity (LPIPS) score~\cite{lpips:conf/cvpr/ZhangIESW18}. 

Statistically, \textbf{MSE} calculates the average squared difference on a pixel level between the reconstructed and original images. \textbf{PSNR} relates this \textbf{MSE} to the maximum pixel values, essentially considering the ratio of the maximal value to \textbf{MSE} in a logarithmic manner. 

For more modern visual assessments, \textbf{SSIM} mimics the human visual system to measure the structural variance of images based on luminance, contrast, and structure. \textbf{LPIPS} determines the perceptual similarity between the original and reconstructed images by learning the inverse mapping from the generated image back to the original. For MSE and LPIPS, lower values indicate greater similarity, whereas for SSIM and PSNR, higher values signify closer resemblance.

\section{Motivation study}

To motivate the study of our gradient inversion for diffusion models, we conduct an exploratory experiment below on data reconstruction by approximating the gradients. This experiment compares the gradient inversion depending on whether the server or clients initialize $\{\epsilon, t\}$, on $32 \times 32$ \textit{Cifar-10} dataset.

\begin{figure}[th!]
	\centering
 \subfigure[original]{	\includegraphics[width=0.15\linewidth]{"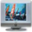"}
 \label{subfig:original}
 } 
 \hfill
 \subfigure[dummy-origin]{	\includegraphics[width=0.15\linewidth]{"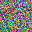"}
 \label{subfig:dummy}
 }
 \hfill
 \subfigure[server-init]{	\includegraphics[width=0.15\linewidth]{"imgs/dummy_image_idx_10086_iter_200_knownt&e.png"}
 \label{subfig:server_init}
 }
 \hfill
 \subfigure[client-init]{	\includegraphics[width=0.15\linewidth]{"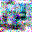"}
 \label{subfig:client_init}
 }
 \caption{Reconstruction visualization on \textit{Cifar-100} (size $32 \times 32$) for 200 iterations. \ref{subfig:original} and \ref{subfig:dummy} are the original training data and the random dummy initialization of the same size image. \ref{subfig:server_init} shows the reconstructed image by the server when $\{\epsilon, t\}$ are known and \ref{subfig:client_init} shows the results when the client samples $\{\epsilon, t\}$, where the adversarial server needs to randomly initialize them for inversion.}
  \label{fig:who_initialze_et}
 \end{figure}

From Fig.~\ref{fig:who_initialze_et}, we can clearly observe that the training data of diffusion models via known $\{\epsilon, t\}$ pairs can be easily recovered within 200 iterations to optimize dummy data by approximating gradient. However, when the client privately initializes $\{\epsilon, t\}$, the system is shown to be more private-preserving, as by the significant difference between the original and recovered image. Additionally, client initialization saves transmission bandwidth for multiple rounds of communication, especially with data-intense training tasks.

\section{Experimental results}

\subsection{Step-by-step output of two phases for \alg}

% \begin{figure}
%     \centering
%     \includegraphics[width=1.0\textwidth]{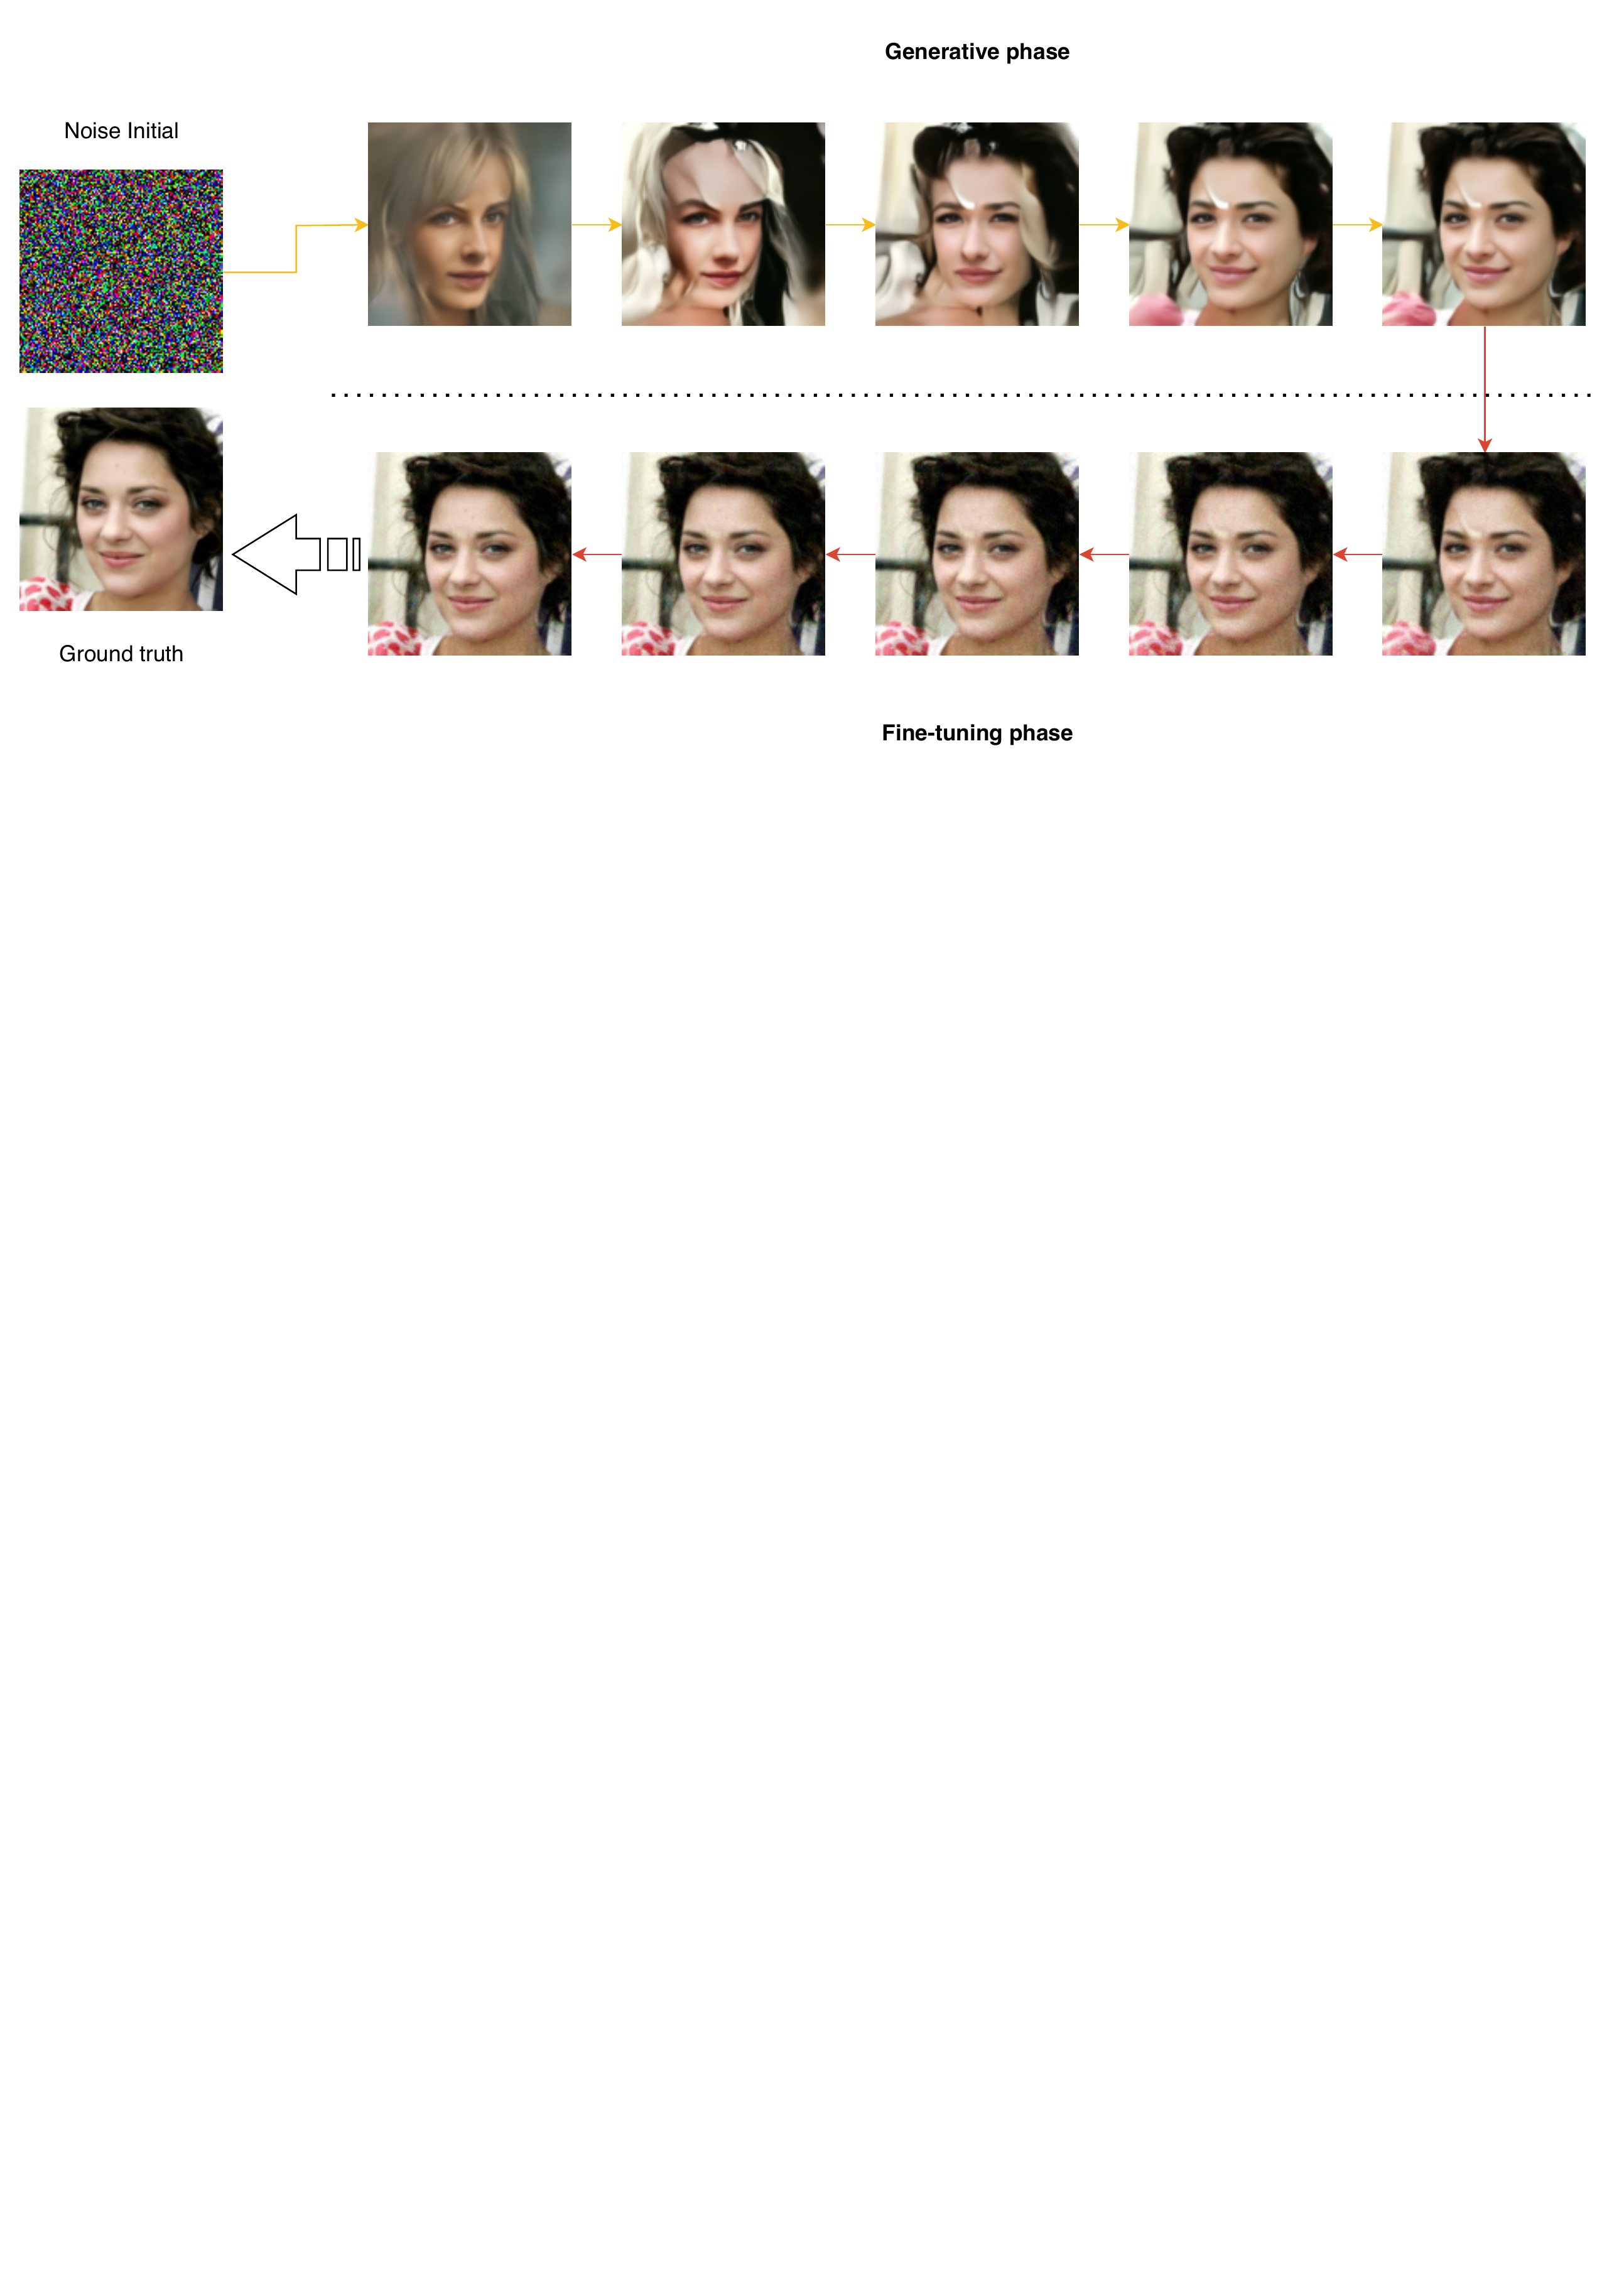}
%     \caption{Intermediate output example for two phases of \alg}
%     \label{fig:enter-label}
% \end{figure}

\begin{figure}
    \centering
    \includegraphics[width=1.0\textwidth]{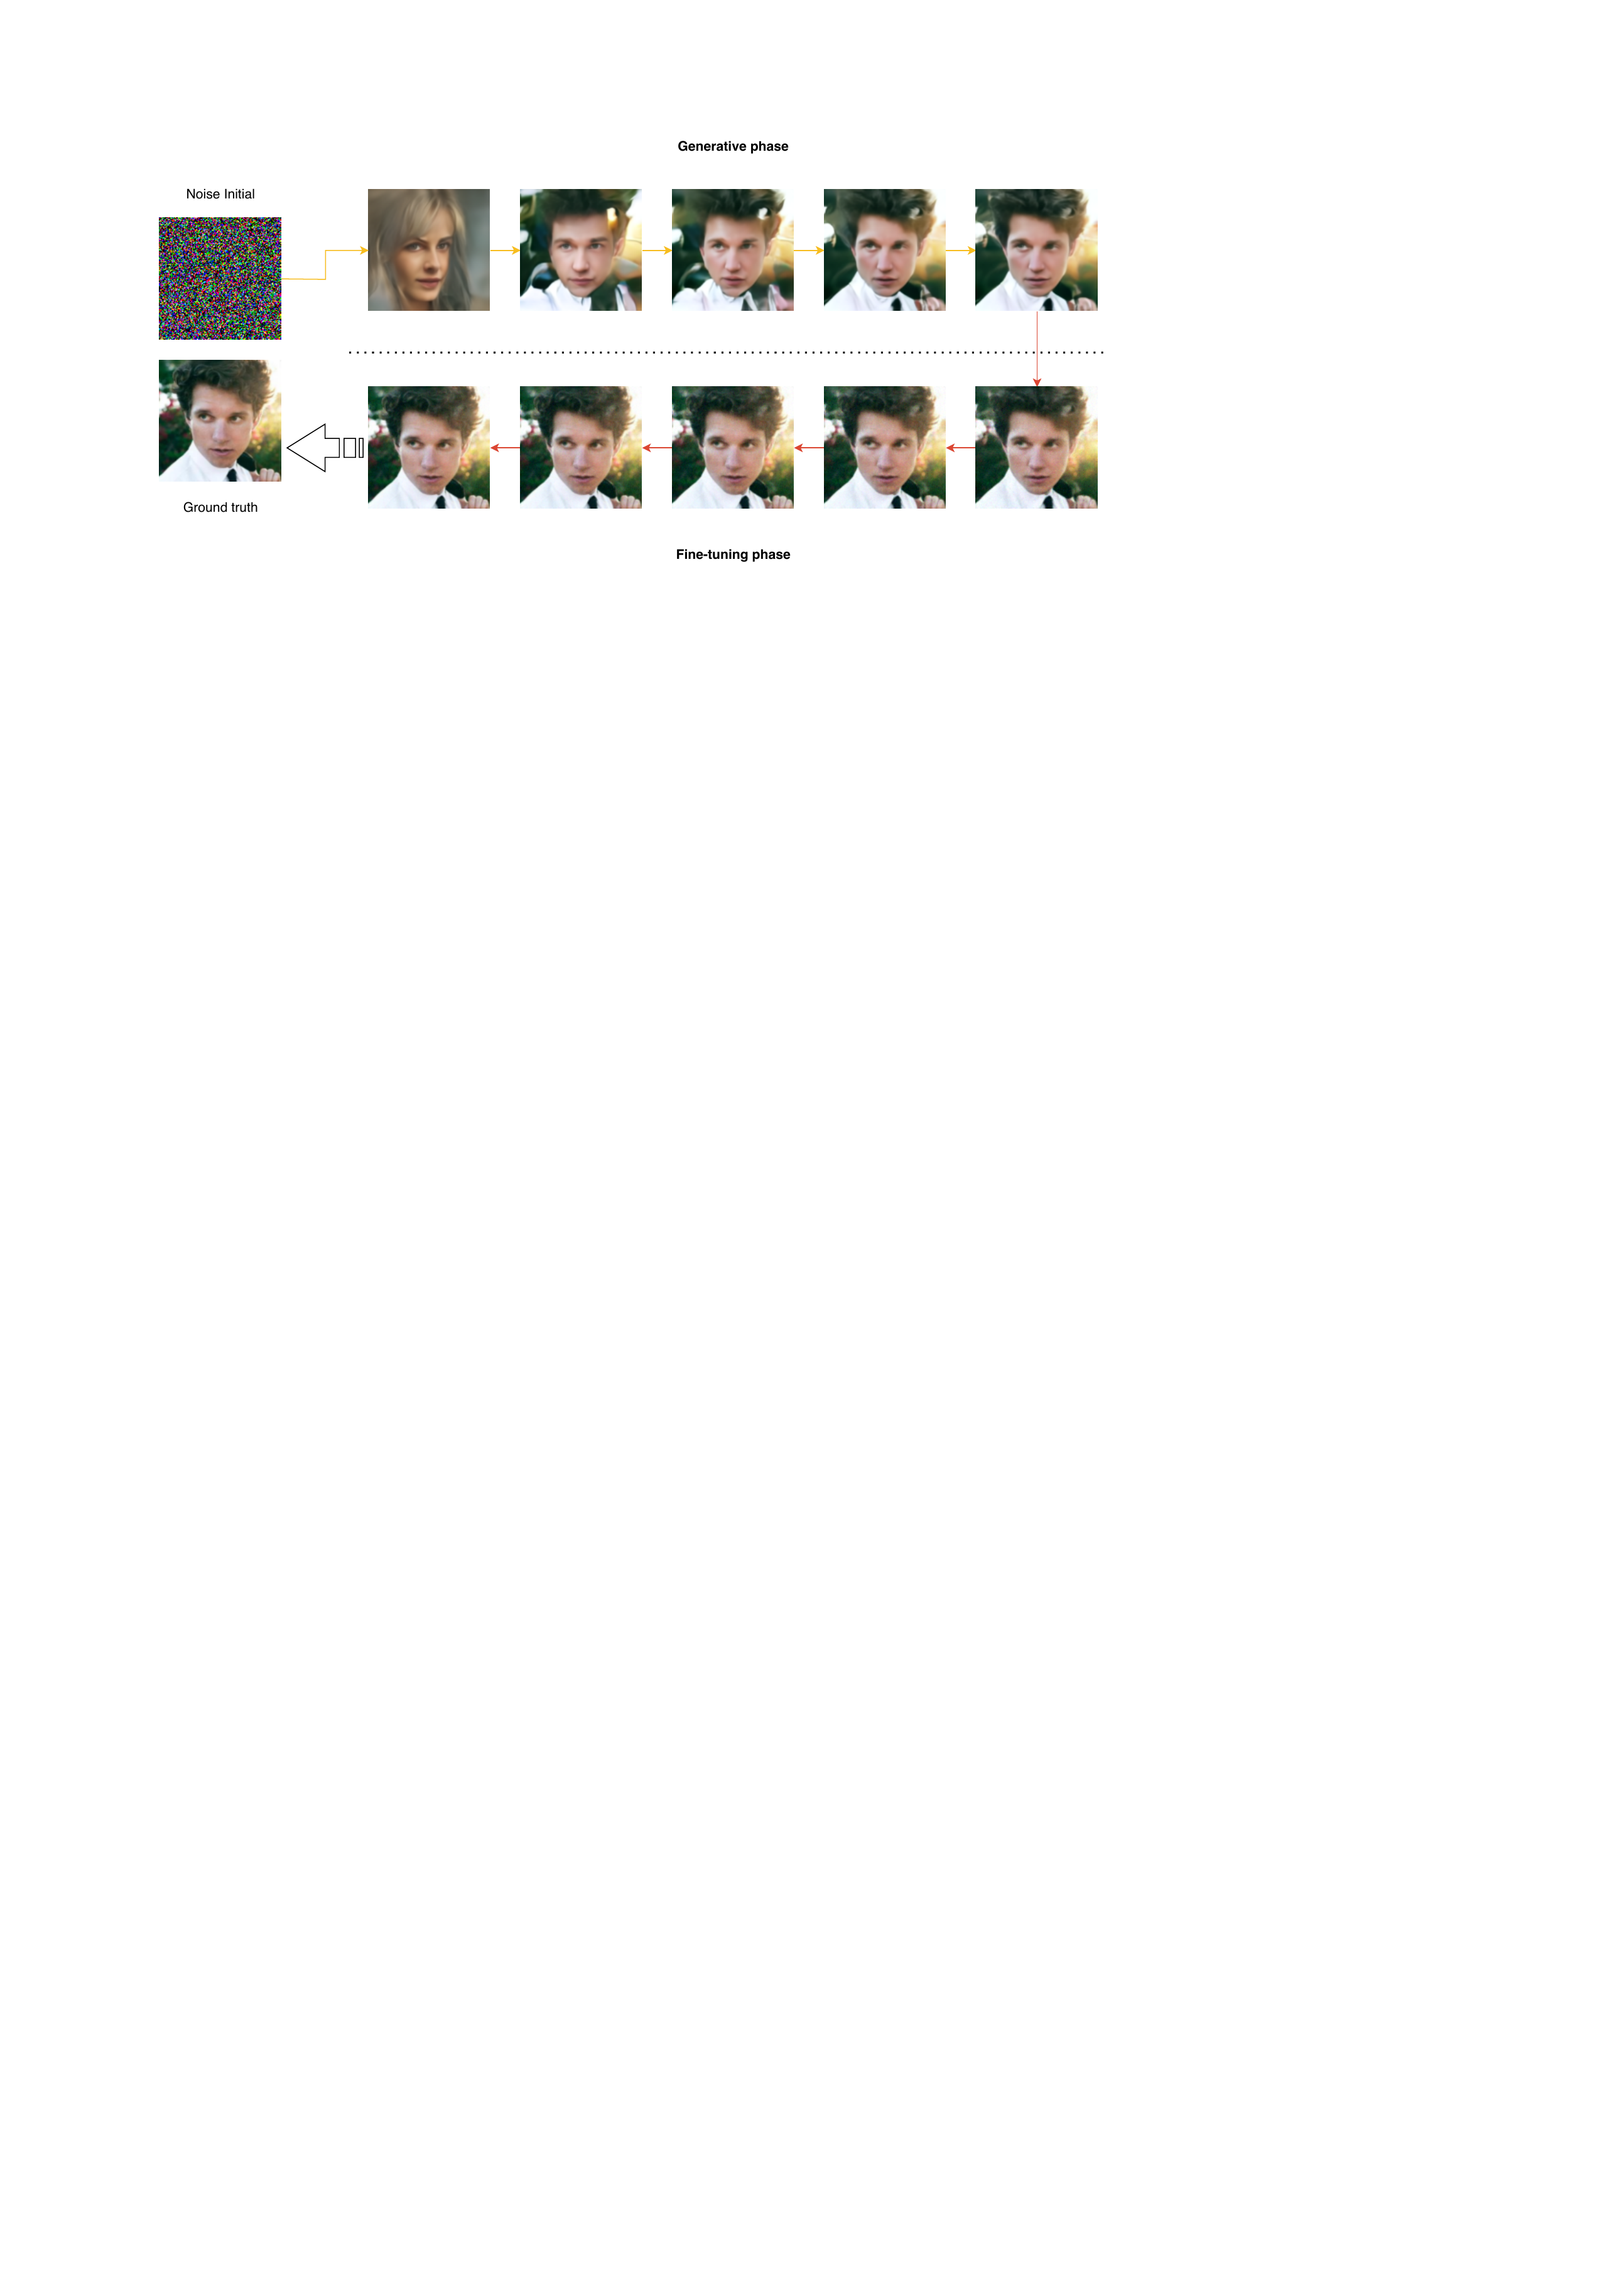}
    \caption{Intermediate output example for two phases of \alg}
    \label{fig:enter-label}
\end{figure}

\begin{figure}
    \centering
    \includegraphics[width=1.0\textwidth]{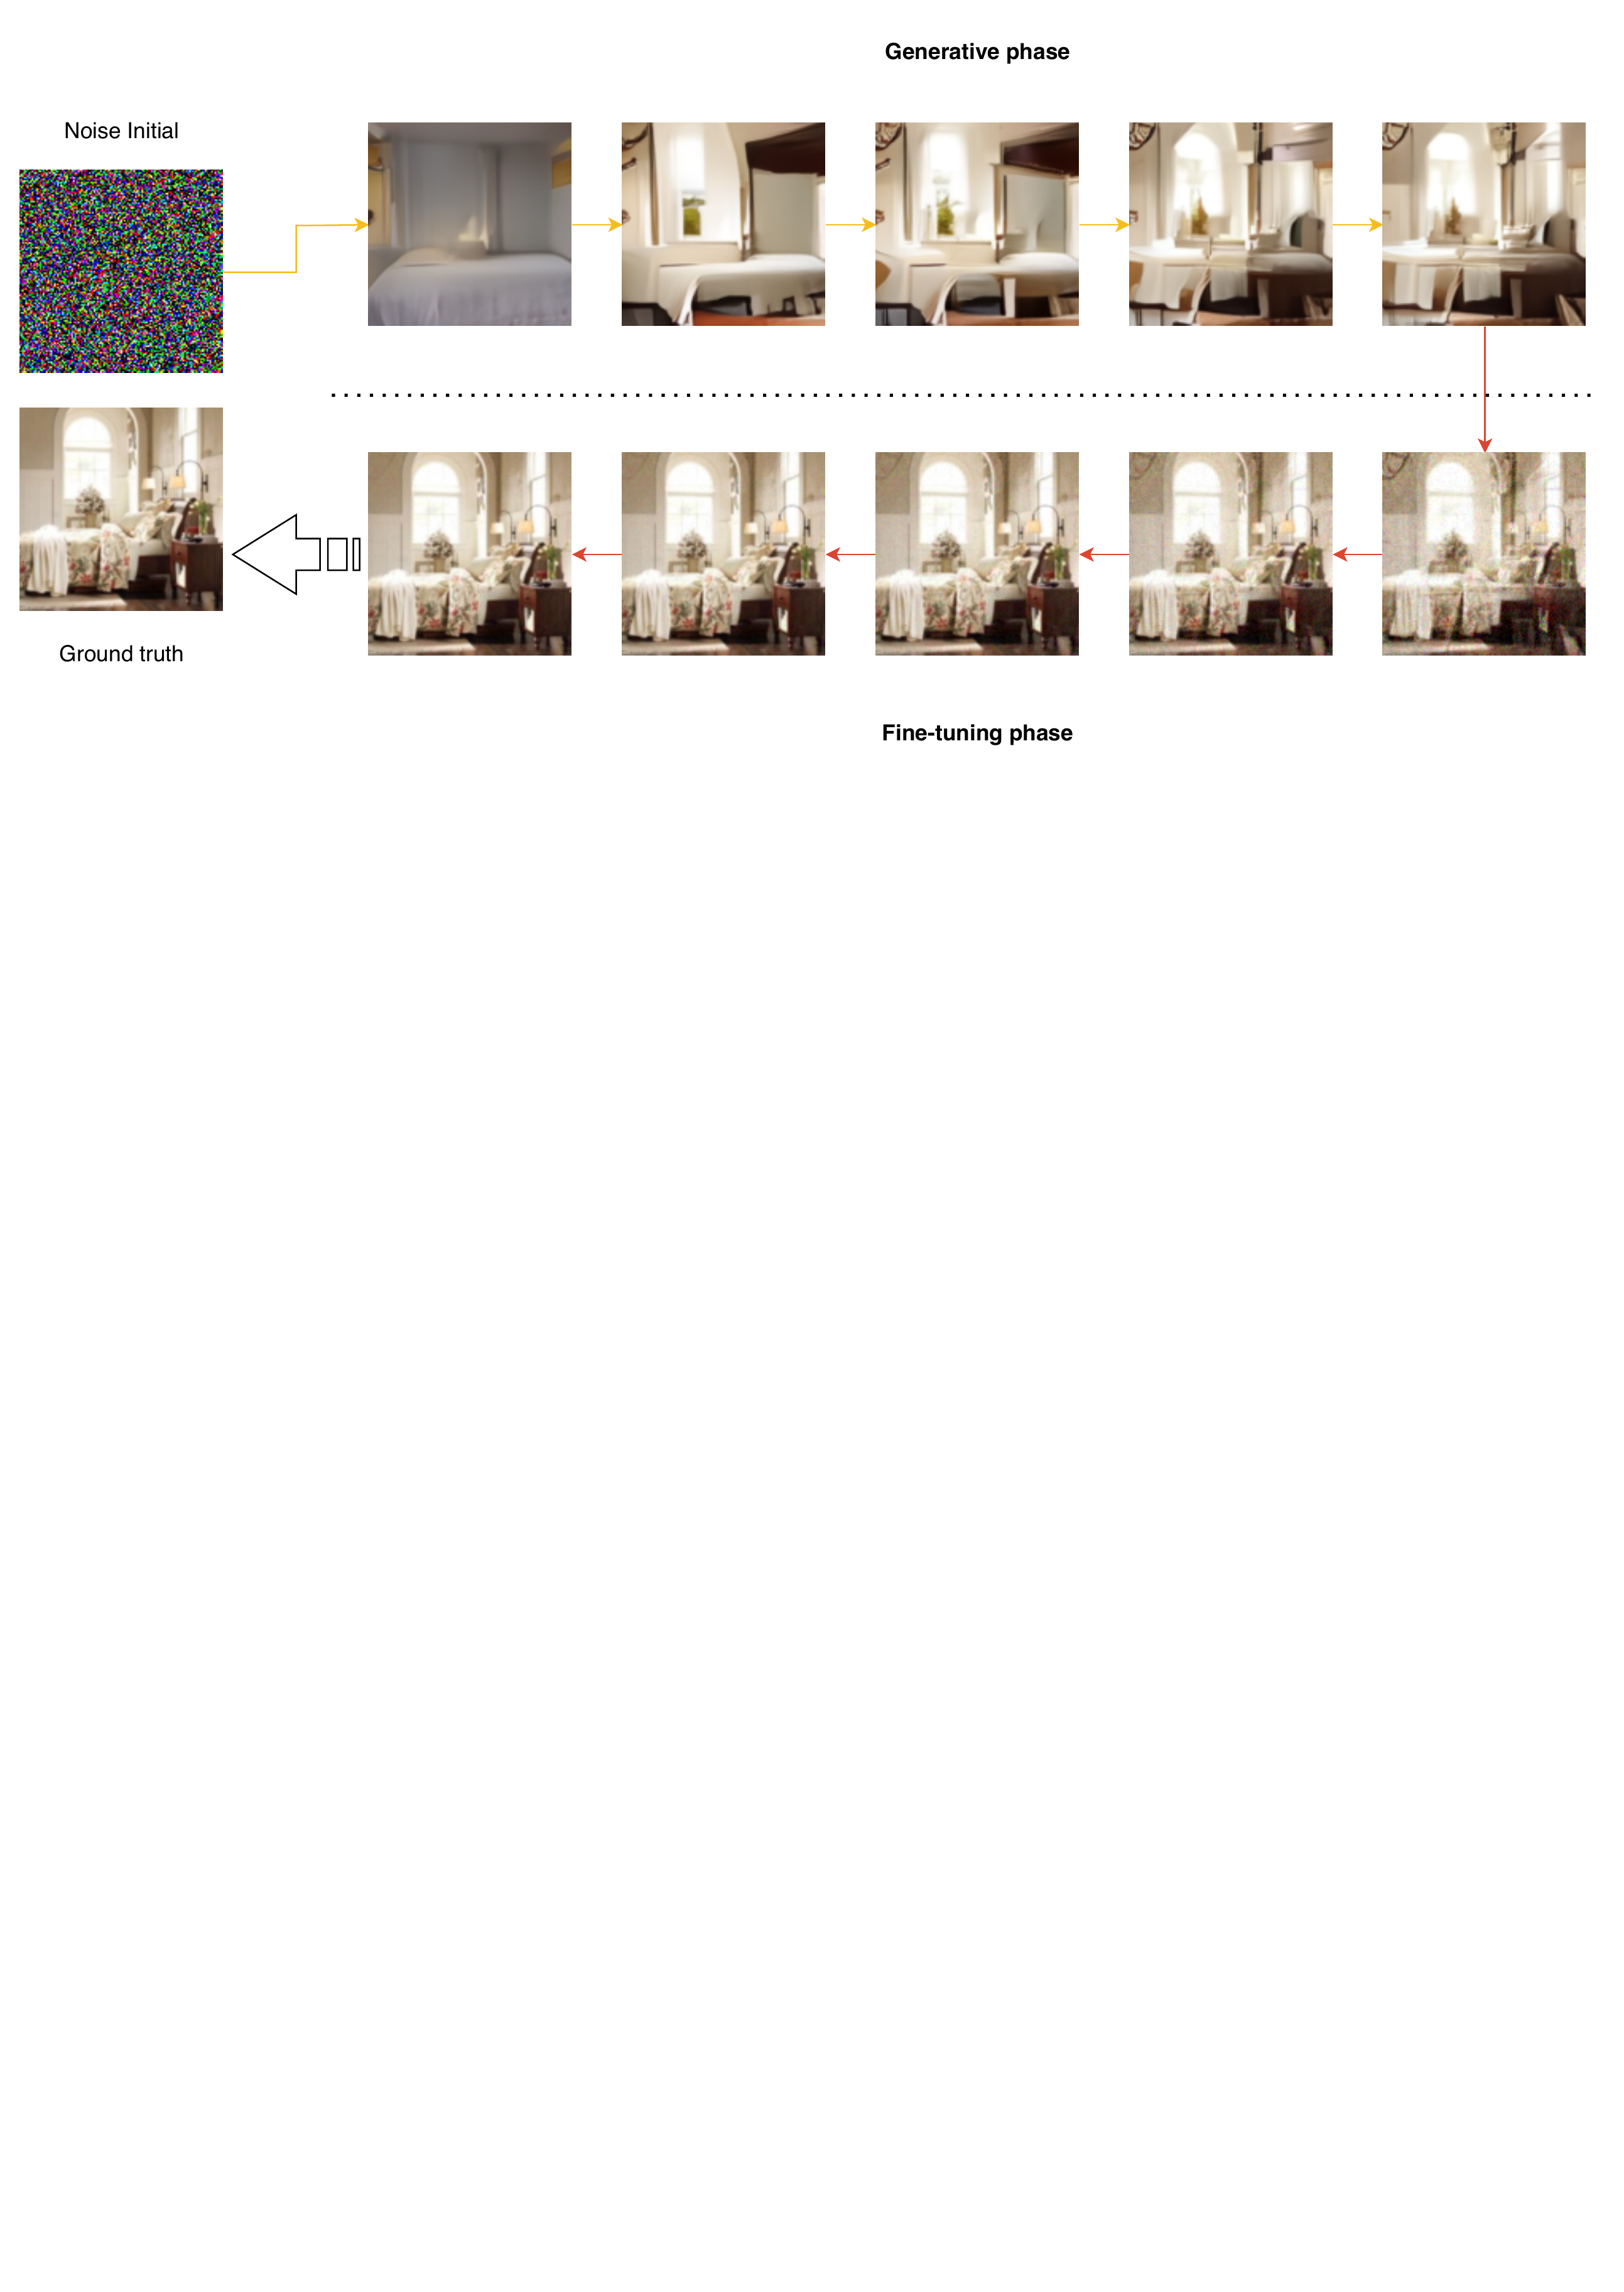}
    \caption{Intermediate output example for two phases of \alg}
    \label{fig:enter-label}
\end{figure}

\begin{figure}
    \centering
    \includegraphics[width=1.0\textwidth]{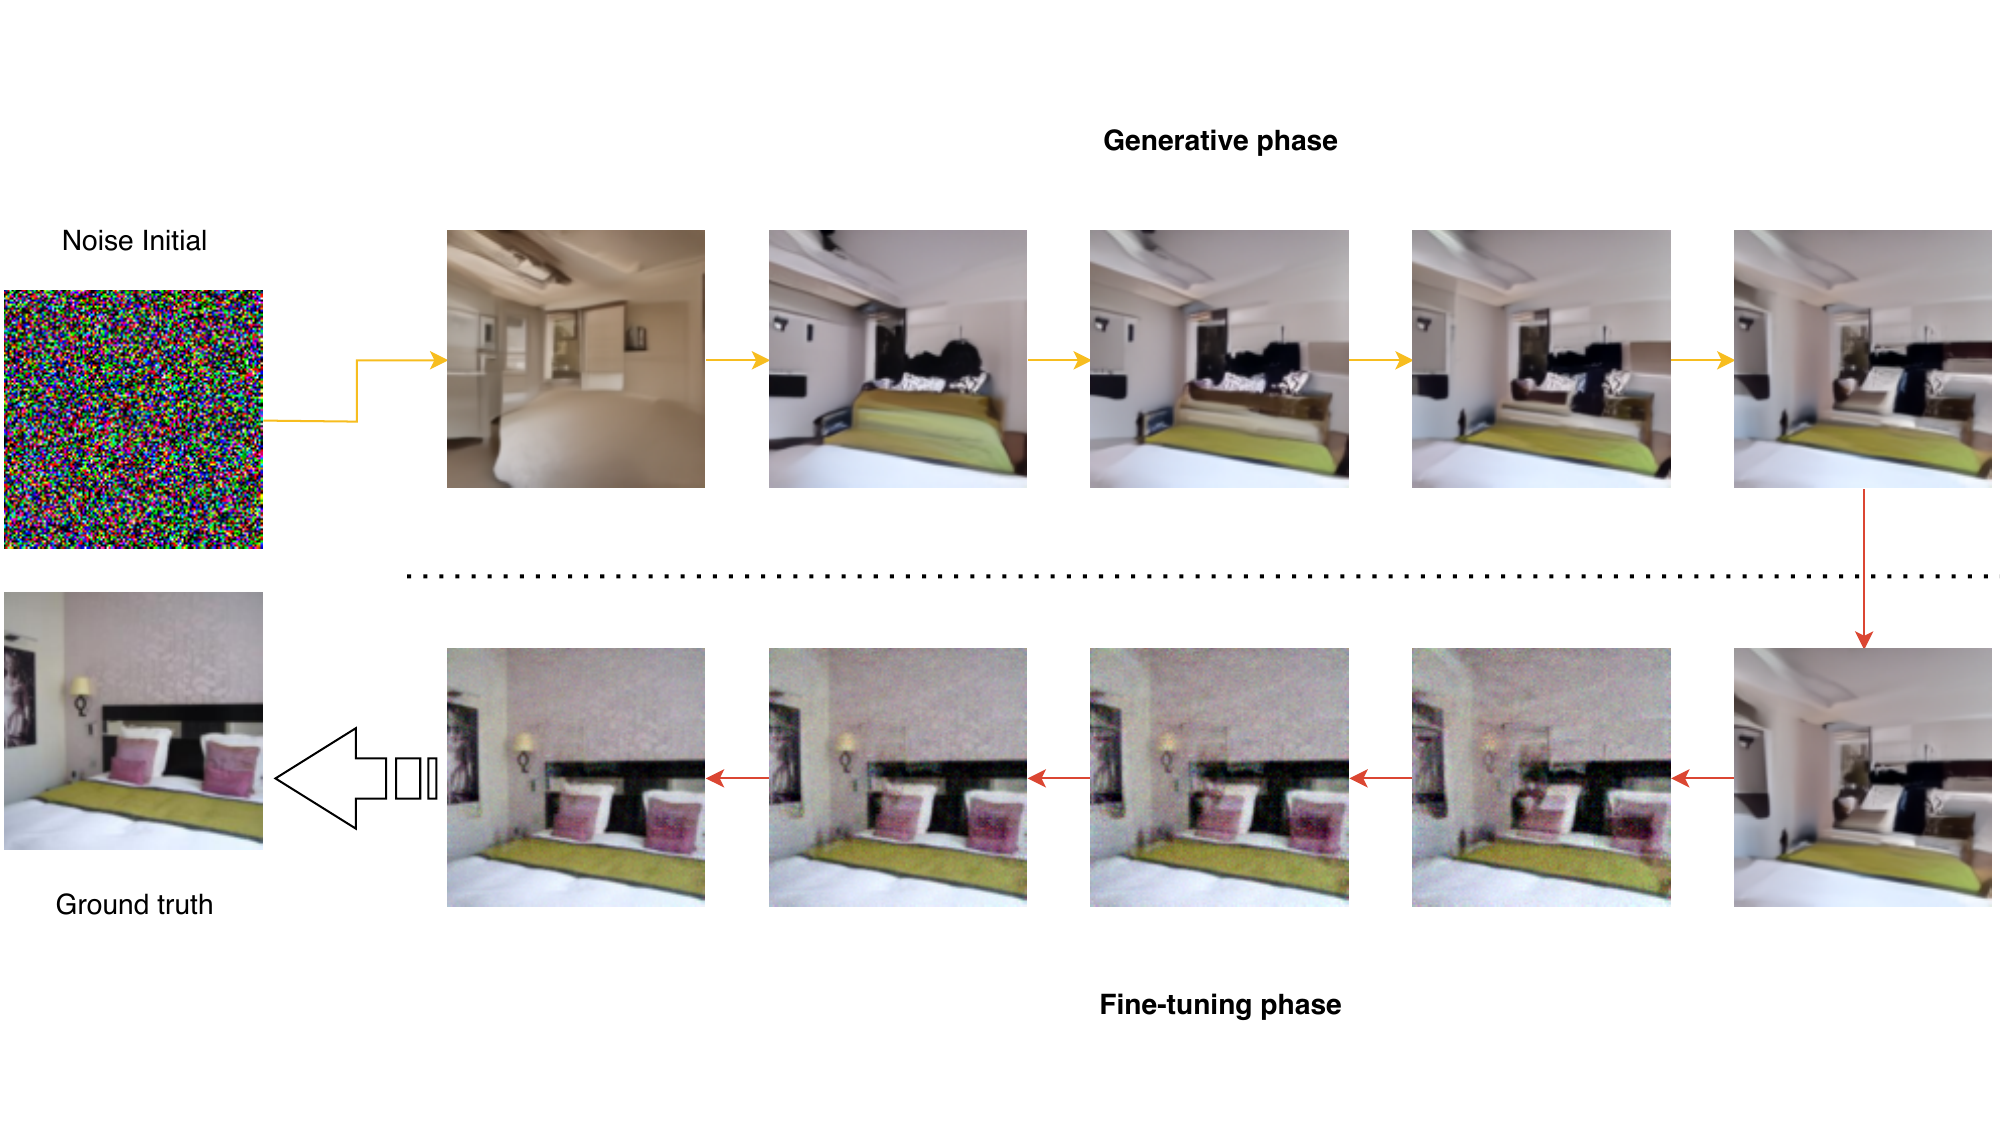}
    \caption{Intermediate output example for two phases of \alg}
    \label{fig:enter-label}
\end{figure}
